# Supplementary material for: Information Theoretic Representation Distillation
Source: arXiv:2112.00459 source file (2022-10-07)
Supplement: Supplementary file 1 [file costs.tex]

\small
\begin{tabular}{c|ccc}
    \toprule
    v.s. & ReviewKD & CRCD & HSAKD \\
    \midrule
    Memory & $\bf{4.08 \times}$ & {\color{red} over GPU (24GB) limit} & $\bf{5.61 \times}$\\
    Train time & $\bf{2.22 \times}$ & $\bf{4.00 \times}$ & $\bf{31.06 \times}$\\
    \midrule
\end{tabular}
