# Supplementary material for: Information Theoretic Representation Distillation
Source: arXiv:2112.00459 source file (2022-10-07)
Supplement: Supplementary file 2 [file kernels.tex]

% RN50 - MN2 - ABLATION [mu, std]
% Poly -> [71.22, 71.52, 71.83] -> [71.52, 0.25]

% a=1.50
% h=1.0 -> [71.17, 71.31, 70.95] -> [71.14, 0.18]
% h=5.0 -> [71.03, 71.03, 70.90] -> [70.99, 0.08]

% a=1.01 [wrong as should be 1.50]
% h=5.0 -> [70.89] -> []

\resizebox{.60\linewidth}{!}{\begin{tabular}{c|ccc}
    \toprule
    % & & \multicolumn{2}{c}{RBF} \\
    % \cline{3-4}
    $\kappa$ & Polynomial & RBF ($\sigma\approx1.0$) & RBF ($\sigma\approx5.0$) \\
    \midrule
    Mean & 71.52 & 71.14 & 70.99 \\
    Std & 0.25 & 0.18 & 0.08 \\
    \midrule
\end{tabular}}
