# Supplementary material for: Information Theoretic Representation Distillation
Source: arXiv:2112.00459 source file (2022-10-07)
Supplement: Supplementary file 3 [file log_mi.tex]

% RN50 - MN2 - ABLATION [mu, std]
% Gs - Gst -> [71.22, 71.52, 71.83] -> [71.52, 0.25]
% Gs / Gst -> [] -> []
% log(Gs) - log(Gst) -> [70.98, 71.44, 71.66] -> [71.36, 0.35]

% $G_s / G_{st}$
\resizebox{.45\linewidth}{!}{\begin{tabular}{ccc}
    \toprule
    $\mathcal{L}_{mi}$ & $G_s-G_{st}$  & $log_2(G_s)-log_2(G_{st})$ \\
    \midrule
    Mean & 71.52 & 71.36 \\
    Std & 0.25 & 0.35 \\
    \midrule
\end{tabular}}
